# Supplementary material for: UniEP: Unified Expert-Parallel MoE MegaKernel for LLM Training
Source: arXiv:2604.19241 source file (2026-04-21)
Supplement: Supplementary file 1 [file appendix.tex]

\section{Hello World}
%\subsection{Hello World}
